# Supplementary material for: Convolutional Phase Retrieval via Gradient Descent
Source: arXiv:1712.00716 source file (2019-10-06)
Supplement: Supplementary file 1 [file appendix.tex]

\section{Spectral Norm of Partial Random Circulant Matrix}

\section{Elementary Tools and Results}
